# Supplementary material for: Face Recognition: Too Bias, or Not Too Bias?
Source: arXiv:2002.06483 source file (2020-04-21)
Supplement: Supplementary file 1 [file supplemental.tex]

\newpage
\onecolumn

% \begin{minipage*}[\linewidth]{width of the minipage}
% \renewcommand{\thesection}{\alph{section}}
\glsresetall

\begin{table}
\begin{center}
\glsunsetall
\caption{Intended \gls{fpr} per subgroup. Each tuple represents percentage the respective rate was achieved (\textcolor{green}{+\%} or \textcolor{red}{-\%}) paired with FNR. Each subgroup shows the use of $t_g$ (top) and individual $t_o$ (bottom).}
\begin{tabular}{l c c c c c}
     \gls{fpr} & 0.3 & 0.1 & 0.01 & 0.001 & 0.0001\\\midrule
    \multirow{2}{.1mm}{\textbf{\gls{af}}} & (\textcolor{red}{-4.5}, )&(\textcolor{red}{-13.4}, )  &(\textcolor{red}{-25.8}, ) &(\textcolor{red}{-25.8}, )  &(\textcolor{red}{-25.5}, )  \\[-4pt]
        & (0.0, ) &(0.0, )  & (0.0, ) &  (\textcolor{green}{0.1}, )&(\textcolor{red}{-5.6}, )  \\[-1pt]
        
    \multirow{2}{3mm}{\textbf{\gls{am}}}&(\textcolor{green}{2.3}, )&(\textcolor{green}{4.1}, )&(\textcolor{green}{11.2}, )&(\textcolor{green}{14.5}, )&(\textcolor{green}{52.1}, ) \\[-4pt]
        & (0.0, ) &(0.0, )  & (\textcolor{green}{0.2}, ) & (\textcolor{green}{0.2}, ) & (\textcolor{red}{5.4}, )\\[-1pt]
        
    \multirow{2}{3mm}{\textbf{\gls{bf}}}& (\textcolor{red}{-1.6}, ) &(\textcolor{red}{-8.2}, ) &(\textcolor{red}{-23.4}, ) &(\textcolor{red}{-27.7}, ) &(\textcolor{red}{-41.8}, ) \\[-4pt]
        & (0.0, ) &(\textcolor{red}{-0.1}, )  & (0.0, ) & (0.0, ) & (\textcolor{red}{5.7}, )\\[-1pt]
        
    \multirow{2}{3mm}{\textbf{\gls{bm}}}&(\textcolor{green}{2.3}, )&(\textcolor{green}{6.5}, )&(\textcolor{green}{17.6}, )&(\textcolor{green}{29.8}, )&(\textcolor{green}{95.8}, ) \\[-4pt]
        & (0.0, ) &(\textcolor{red}{-0.1}, )  & (0.0, ) & (\textcolor{green}{0.1}, ) & (\textcolor{red}{5.5}, )\\[-1pt]
        
    \multirow{2}{3mm}{\textbf{\gls{if}}} &(\textcolor{red}{-9.0}, ) &(\textcolor{red}{-26.1}, ) &(\textcolor{red}{-58.6}, ) &(\textcolor{red}{-46.1}, ) &(\textcolor{red}{-60.9}, )\\[-4pt]
        & (0.0, ) &(0.0, )  & (0.0, ) & (\textcolor{green}{0.2}, ) & (\textcolor{red}{5.4}, )\\[-1pt]
        
    \multirow{2}{3mm}{\textbf{\gls{im}}} &(\textcolor{green}{2.4}, )&(\textcolor{green}{4.3}, )&(\textcolor{red}{-3.4}, )&(\textcolor{red}{-16.4}, )&(\textcolor{red}{-76.2}, )\\[-4pt]
        & (0.0, ) &(0.0, )  & (\textcolor{green}{0.1}, ) & (\textcolor{green}{0.1}, )  &(\textcolor{red}{5.5}, ) \\[-1pt]
        
    \multirow{2}{3mm}{\textbf{\gls{wf}}} &(\textcolor{red}{-1.1},) &(\textcolor{green}{5.8}, ) &(\textcolor{green}{50.6}, ) &(\textcolor{green}{52.6}, ) &(\textcolor{green}{158.0}, )\\[-4pt]
       & (0.0, ) &(\textcolor{red}{-0.1}, )  & (\textcolor{green}{0.3}, ) & (\textcolor{green}{0.2}, )  &(\textcolor{red}{5.5}, )  \\[-1pt]

    \multirow{2}{3mm}{\textbf{\gls{wm}}} & (\textcolor{green}{10.5}, ) & (\textcolor{green}{38.6}, )& (\textcolor{green}{120.0}, )& (\textcolor{green}{83.4}, )& (\textcolor{green}{200.0}, ) \\[-4pt]
    
        & (0.0, ) &(\textcolor{green}{0.2}, ) &(\textcolor{green}{0.2}, ) & (\textcolor{green}{0.2}, )&(\textcolor{red}{-5.5}, )\\[-1pt]
    % \midrule
    % \multirow{2}{3mm}{\textbf{Avg.}} \\[-4pt]
    %   & (0.0, ) &(0.0, )  & (\textcolor{green}{-}, ) &  \\[-10pt]
\end{tabular}
\end{center}
\end{table}

\begin{figure}
    \centering
    \includegraphics[width=\textwidth]{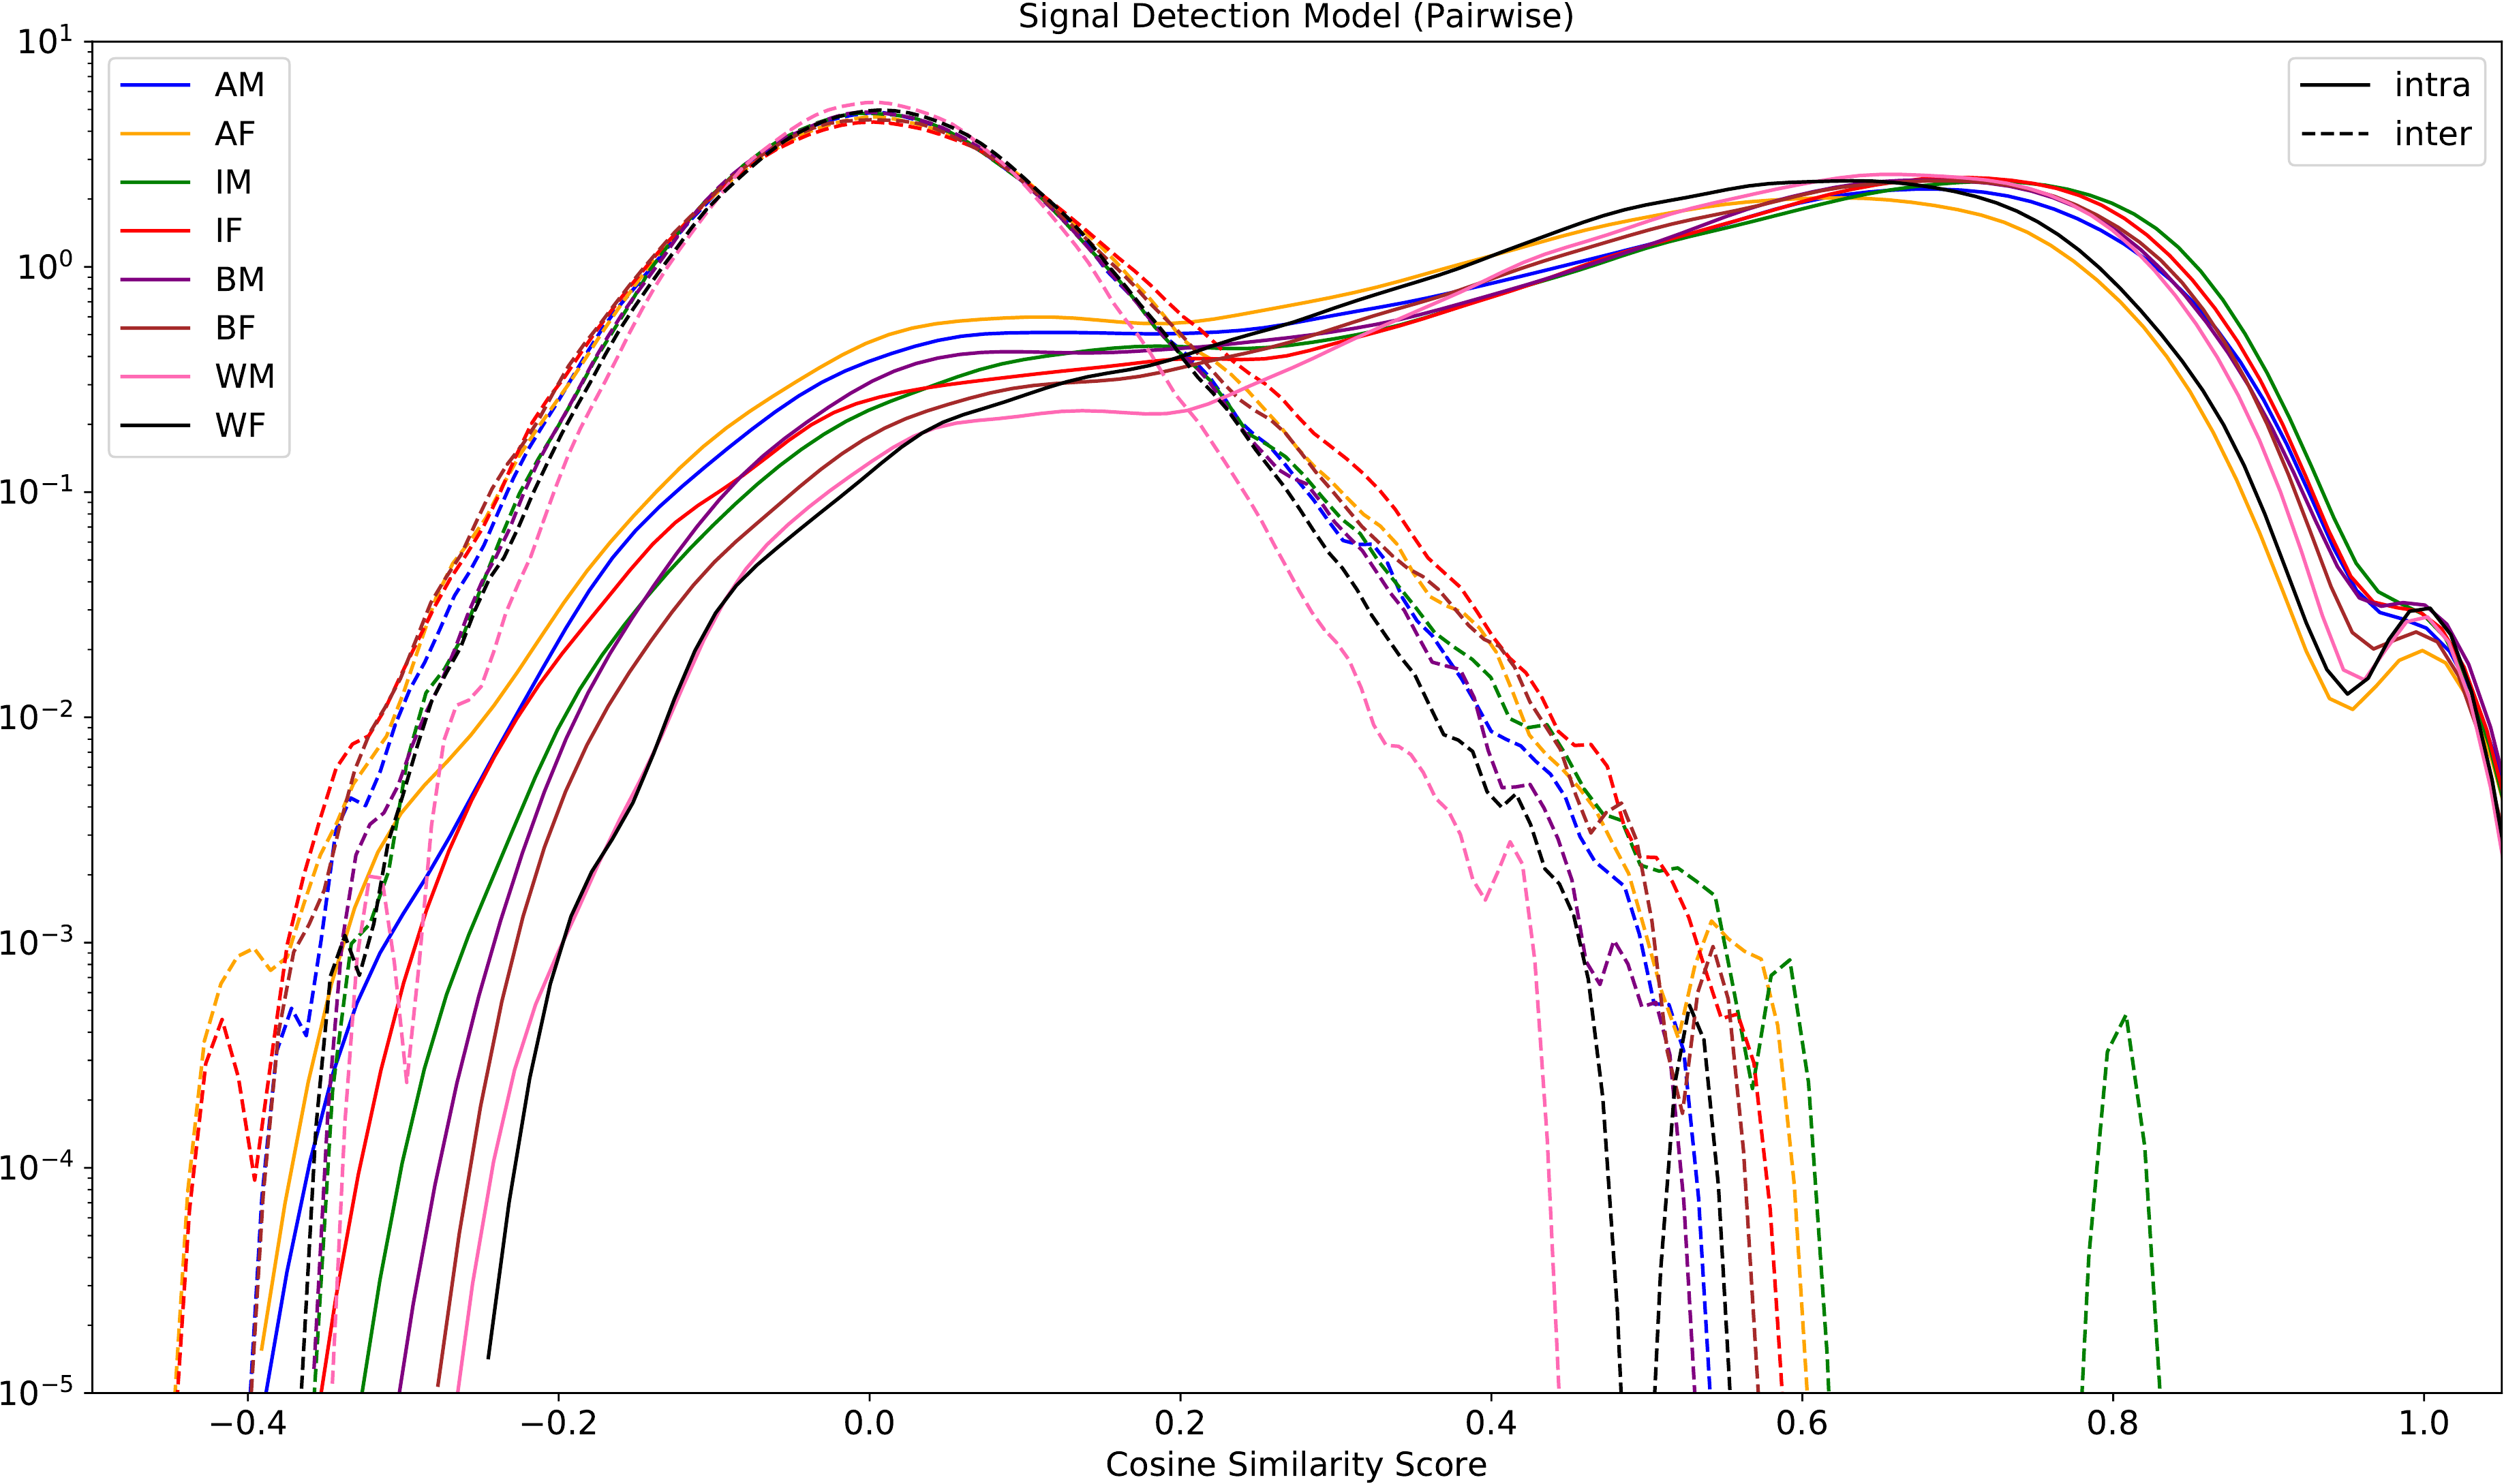}
    \caption{Caption}
    \label{fig:my_label}
\end{figure}

Sample faces per subgroup of the \gls{bfw} dataset are shown in Fig.~\ref{fig:montage:app}.
\begin{figure}[h!]
    \centering
    \includegraphics[width=.7\linewidth]{figures/facemontage.pdf}
    \caption{\textbf{Sample of \gls{bfw}}. Each row depicts a different gender, \gls{f} (top) and \gls{m} (bottom). Columns are grouped by ethnicity (\ie \gls{a}, \gls{b}, \gls{i}, and \gls{w}, respectfully).}
    \label{fig:montage:app}
\end{figure}
\begin{comment}
\scriptsize

\end{comment}

% \end{minipage*}
